# Supplementary material for: Enhanced Conductivity Along Lateral Homojunction Interfaces of Atomically Thin Semiconductors
Source: arXiv:1612.03921 ancillary file (2016-12-12)
Supplement: Supplementary file 1 [file Jia_2016_Supplementary.pdf]

# Supplementary Information for Enhanced Conductivity Along Lateral Homojunction Interfaces of Atomically Thin Semiconductors

Ying Jia, Teodor K. Stanev, Erik J. Lenferink, Nathaniel P. Stern
*Department of Physics and Astronomy, Northwestern University, Evanston, IL, US 60208*

### S1. $I_{sd} - V_{sd}$ Characteristics of $MoS_2$ Devices

In this section, we show the $I_{sd} - V_{sd}$ characteristics of the devices shown in Fig. 1c and Fig. 3b in the main text. Linear $I_{sd} - V_{sd}$ curves are observed in all the devices, confirming Ohmic contacts.

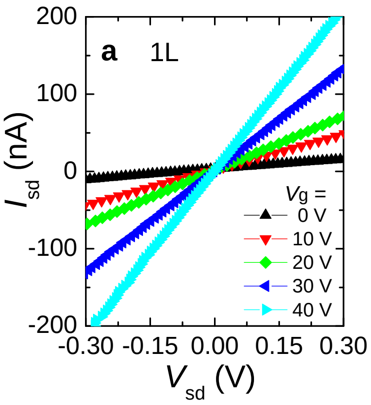


FIG. S1. $I_{sd} - V_{sd}$ curves at various gate voltages for the 1L and the ML devices shown in Fig. 1c in the main text.

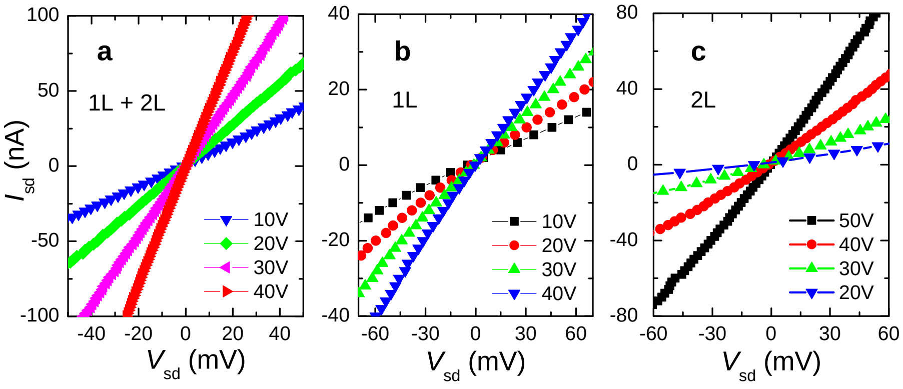


FIG. S2. $I_{sd} - V_{sd}$ curves at various gate voltages for the two-terminal devices shown in the inset of Fig. 3b in the main text. From left to right, the curves are for the 1L+2L, the 1L and the 2L devices.

### S2. Low Temperature Resistivity

In this section, we present the gate-dependent effective conductivity of an additional 1L+2L device, together with its low temperature effective resistivity $\frac{1}{\sigma_{\mathrm{eff}}} = \frac{W}{GL}$.

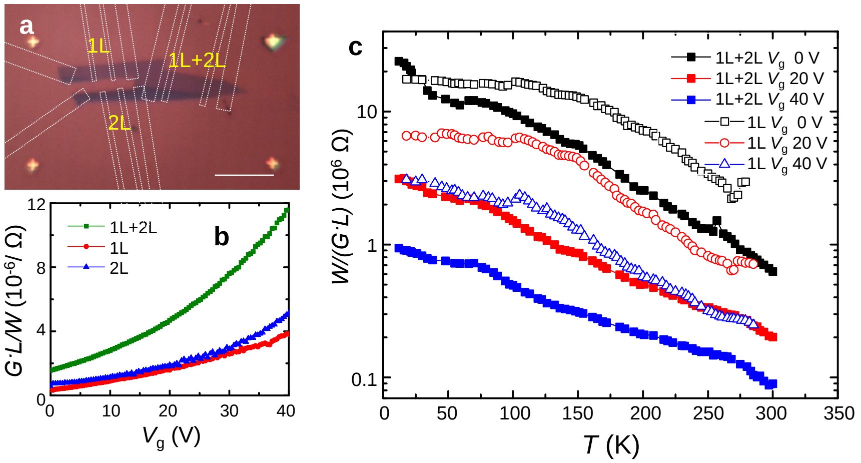


FIG. S3. **a** Optical image of a 1L/2L $MoS_2$ flake shaped by RIE etching. The white doted lines mark the electric contacts. The scale bar is 10 $\mu$m. **b** Gate-voltage-dependent conductivities of the 1L, the 2L and the 1L+2L devices at room temperature. **c** Resistivity as a function of temperature for the 1L and the 1L+2L devices in semi-log scale.

Fig. S3 shows an optical image of the 1L+2L flake. At room temperature, the 1L+2L device exhibits enhanced effective conductivity and effective mobility $\mu_{\text{FE-eff}} = 31.1$ cm$^2$/Vs (mobilities of the 1L and the 2L devices are 16.1 cm$^2$/Vs and 8.6 cm$^2$/Vs, respectively). At low temperature, the higher effective conductivity (lower effective resistivity) over the 1L device is retained. The effective resistivity of the 1L+2L device increases with reducing temperature. The semiconductor behavior suggests that, unlike the 2DEG in $Al_xGa_{1-x}As$/GaAs, the Fermi level is still lower than the conduction band minimum at the 1L/ML interface. The temperature dependence of the 1L resistivity is consistent with Ref. [1]. For each gate voltage, the effective resistivity of the interface samples generally remains lower than the bare monolayer across the temperature range (i.e. the enhanced effective conductivity persists).

## S3. Summary of the Measured $MoS_2$ Devices

In this section, we summarize all the measured $MoS_2$ devices. All the 1L+ML devices exhibit enhanced effective conductivity and effective field-effect mobility over their independent 1L and ML channels.

TABLE S1. Summary of measured $MoS_2$ devices.

| Sample No. | Image | Contact number | Layer number | $\sigma_1$, $\sigma_{\text{m}}$ and $\sigma_{\text{eff}}$ at $V_{\text{g}} = 40$ V ($10^{-6}/\Omega$) | $\mu_{\text{FE-1}}$, $\mu_{\text{FE-m}}$ and $\mu_{\text{FE-eff}}$ (cm$^2$/Vs) |
|---|---|---|---|---|---|
| 1 | Fig. 1c | 4 | 1L | 1.23 | 4.1 |
| | | 4 | 8L | 4.53 | 11.4 |
| | | 4 | 1L+8L | 7.87 | 20.2 |
| 2 | Fig. 3b | 2 | 1L | 1.32 | 2.8 |
| | | 2 | 2L | 2.57 | 11.0 |
| | | 2 | 1L+2L | 4.41 | 15.2 |
| 3 | Fig. S3a | 4 | 1L | 3.83 | 8.6 |
| | | 4 | 2L | 5.14 | 16.1 |
| | | 4 | 1L+2L | 11.58 | 31.1 |

## S4. The Simple Heterostructure Model

We construct a simple heterostructure model to interpret the electrical properties along the interface. Other possible explanations of the enhanced effective conductivity and effective mobility such as edge states are not excluded by the measurements. In our model, the carrier transfer from the 1L side to the ML side (Fig. S4a) is only determined by potential difference. Carrier transfer between different points in $k$ space is assisted by phonons and is complete when the system reaches thermal equilibrium. We use a traditional semiclassical model of a semiconductor heterostructure that is necessarily a simplified treatment. A more detailed theoretical analysis of the homojunction devices is beyond the scope of our experimental study, but it would be welcomed.

We first obtain the necessary parameters for the model, the carrier densities in 1L and ML $MoS_2$; we then discuss the equations that we solve for the parameters of the interface state, including the width of the accumulation region and the carrier density at the interface. Finally, the estimated mobilities of interface electrons, assuming they are confined to this accumulation region, are extracted from the measured conductance of the 1L+ML devices.

### S4.1 Carrier densities in 1L and ML $MoS_2$

The electron carrier density $n$ of 1L and ML $MoS_2$ is extracted from the measured properties of the separate 1L and ML devices. In a field-effect transistor, the majority carrier field-effect mobility $\mu_{\mathrm{FE}}$ can be derived from the slope of the gate-voltage-dependent conductivity $\sigma(V_{\mathrm{g}})$ in the linear regime.

$$\mu_{\mathrm{FE}} = \frac{1}{C_i}\frac{\partial\sigma}{\partial V_{\mathrm{g}}} \tag{1}$$

where $C_{\mathrm{i}}$, the capacitance per unit area, is $1.3\times10^{-4}$ F/m$^2$ for our 285 nm-thick $SiO_2$ layer [2]. The $\mu_{\mathrm{FE}}$ values of the 1L and the ML devices in Fig. 1c are 4.1 cm$^2$/Vs and 11.4 cm$^2$/Vs, respectively.

The conductance of a rectangular sample can be expressed as

$$G = \sigma \times \frac{W}{L} = ne\mu \times \frac{W}{L} \tag{2}$$

where $\mu$ is the carrier drift mobility. With the approximation $\mu_{\mathrm{FE}} \approx \mu$, the carrier density $n$ can be estimated as $(0.9 \sim 1.7) \times 10^{12}$ cm$^{-2}$ for 1L and $(0.2 \sim 1.7) \times 10^{12}$ cm$^{-2}$ for ML depending on the gate voltage. Our values are in good agreement with other reports on $MoS_2$ monolayers and multilayers [3, 4]. The similar $n$ for the 1L and the ML $MoS_2$ is also supported by the fact that the charge doping in a mechanically exfoliated pristine few-layer $MoS_2$ on $SiO_2$/Si mainly originates from the trapped charges and the field-induced charges on the surface of $SiO_2$ [5]. To keep the estimates tractable in the following calculation, we use the midpoint of the range $n = 1.0 \times 10^{12}$ cm$^{-2}$ as an estimate of $n$ for both 1L and ML.

For the 1L+ML device, we assume that the carrier densities of the 1L and ML regions are also $1.0 \times 10^{12}$ cm$^{-2}$ as the three devices are fabricated from the same $MoS_2$ flake.

### S4.2 Width of depletion region and carrier density at the interface

In this part, we solve for the width of the depletion region and the carrier density at the interface. The band diagram and carrier density in a $MoS_2$ monolayer/multilayer homojunction in thermal equilibrium is depicted in Fig. S4. A depletion region is formed on the right (1L) side of the junction and an electron accumulation region on the left (ML) side. Due to the offset in the conduction band at the interface, the accumulated carriers are confined in the ML region.

In Fig. S4, $q\Phi_{\mathrm{m}}$ and $q\Phi_1$ are the work functions of ML and 1L $MoS_2$, which are $4.59 \pm 0.03$ eV and $4.49 \pm 0.03$ eV, respectively [6]. The built-in potential in the junction is

$$qV_{\mathrm{bi}} = E_{\mathrm{Fm}} - E_{\mathrm{F1}} = q\Phi_m - q\Phi_1 \approx 0.10\ eV \tag{3}$$

A similar value of ∼0.08 eV was measured by Kelvin probe force microscopy on a 1L/14L $MoS_2$ flake [7]. In terms of potential drops on the two sides of the junction, $V_{\mathrm{bi}}$ can be expressed as

$$V_{\mathrm{bi}} = \phi_{\mathrm{m}} + \phi_1 \tag{4}$$

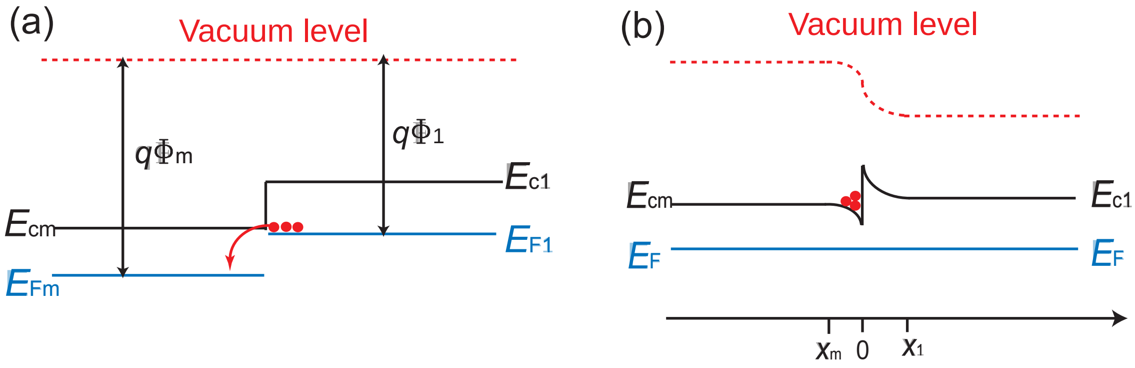


FIG. S4. Band diagram of a $MoS_2$ monolayer/multilayer homo-junction, **a** before and **b** in thermal equilibrium. The left side of each panel presents the bands in multilayer $MoS_2$, the right side is for the monolayer.

The potential drop in the depletion region can be related to the thickness of the depletion region [8]

$$\phi_1 = q\frac{N_{\mathrm{d1}} x_1^2}{2\varepsilon_1} \tag{5}$$

$$V_{\mathrm{bi}} = \phi_{\mathrm{m}} + q\frac{N_{\mathrm{d1}} x_1^2}{2\varepsilon_1} \tag{6}$$

where $x_1$ is the width of depletion region in the 1L $MoS_2$. $N_{\mathrm{d1}}$ is the donor density, which approximately equals the carrier density in $n$-doped $MoS_2$.

In the region $x \leq 0$, we assume that the potential is zero at $x = -\infty$. Using the traditional semiclassical model of a semiconductor, the spatial-dependent carrier density in ML can be written as,

$$n_{\mathrm{m}}(x) = N_{\mathrm{cm}} \exp\left[\frac{E_{\mathrm{F}} - E_{\mathrm{cm}}(x)}{k_{\mathrm{B}}T}\right] = N_{\mathrm{cm}} \exp\left[\frac{E_{\mathrm{F}} - E_{\mathrm{cb}}(-\infty) - q\phi(x)}{k_{\mathrm{B}}T}\right] = N_{\mathrm{cm}} \exp\left[\frac{E_{\mathrm{F}} - E_{\mathrm{cb}}(-\infty)}{k_{\mathrm{B}}T}\right] \exp\left[\frac{q\phi(x)}{k_{\mathrm{B}}T}\right] \tag{7}$$

where $N_{\mathrm{cm}}$ is the density of states.

$$n_{\mathrm{m}}(x) = N_{\mathrm{dm}} \exp\left[\frac{q\phi(x)}{k_{\mathrm{B}}T}\right] \tag{8}$$

where $N_{\mathrm{dm}}$ is the donor density in mulitylayer $MoS_2$.

Poisson's equation for the electric field gives

$$-\varepsilon_{\mathrm{m}}\frac{d^2\phi(x)}{dx^2} = q[N_{\mathrm{dm}} - n_{\mathrm{m}}(x)] = qN_{\mathrm{dm}}\left[1 - \exp\frac{q\phi(x)}{k_{\mathrm{B}}T}\right] \tag{9}$$

$$\Rightarrow \frac{d}{dx}\left(\frac{d\phi}{dx}\right)^2 = 2q\frac{N_{\mathrm{dm}}}{\varepsilon_{\mathrm{m}}}\left[\exp\frac{q\phi(x)}{k_{\mathrm{B}}T} - 1\right]\frac{d\phi}{dx} \tag{10}$$

Integrating from $-\infty$ to 0 using the boundary conditions,

$$\phi(-\infty) = 0 \tag{11}$$

$$\phi(0) = \phi_{\mathrm{m}} \tag{12}$$

gives

$$\left.\left(\frac{d\phi}{dx}\right)^2\right|_{x=0} = \frac{2N_{\mathrm{dm}}k_{\mathrm{B}}T}{\varepsilon_{\mathrm{m}}}\left[\left(e^{\frac{q\phi_{\mathrm{m}}}{k_B T}} - 1\right) - \frac{q\phi_{\mathrm{m}}}{k_{\mathrm{B}}T}\right] \tag{13}$$

$$\Rightarrow E(x)|_{x=0^-} = -\sqrt{\frac{2N_{\mathrm{dm}}k_{\mathrm{B}}T}{\varepsilon_{\mathrm{m}}}}\sqrt{\left(e^{\frac{q\phi_{\mathrm{m}}}{k_B T}} - 1\right) - \frac{q\phi_{\mathrm{m}}}{k_{\mathrm{B}}T}} \tag{14}$$

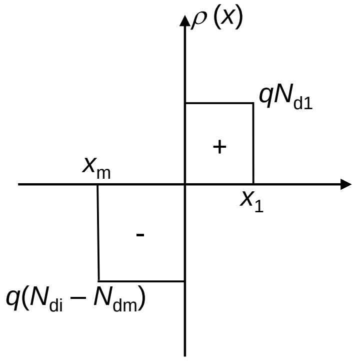


FIG. S5. The net charge density on both side of the junction.

TABLE S2. Calculated parameters of interface electrons.

| $V_{\rm bi}$ (V) | $\phi_{\rm m}$ (V) | $x_1$ (nm) | $x_{\rm m}$ (nm) | $N_{\rm di}$ ($\rm cm^{-2}$) | $\mu_{\rm i}(V_{\rm g}=0\ V)$ ($\rm cm^2/Vs$) | $\mu_{\rm i}(V_{\rm g}=40\ V)$ ($\rm cm^2/Vs$) |
|---|---|---|---|---|---|---|
| 0.05 | 0.035 | 1.0 | 2.9 | $3.9\times10^{12}$ | 2900 | $2.5\times10^4$ |
| 0.1 | 0.052 | 1.2 | 2.3 | $7.7\times10^{12}$ | 1300 | $1.6\times10^4$ |
| 0.15 | 0.064 | 1.3 | 1.9 | $1.2\times10^{13}$ | 970 | $1.1\times10^4$ |

The electric fields on both sides of the junction are related by Gauss's law,

$$\varepsilon_1 E(x)|_{x=0^+} = \varepsilon_m E(x)|_{x=0^-} = -qN_{d1}x_1 \tag{15}$$

$$\Rightarrow \sqrt{2\varepsilon_{\rm m}N_{\rm dm}k_{\rm B}T}\sqrt{\left(e^{\frac{q\phi_{\rm m}}{k_BT}}-1\right)-\frac{q\phi_{\rm m}}{k_{\rm B}T}} = qN_{\rm d1}x_1 \tag{16}$$

In equation (6) and (16), $\varepsilon_1 = 3.43\ \varepsilon_0 = 3.04\times10^{-11}$ F/m and $\varepsilon_{\rm m} = 10.7\ \varepsilon_0 = 9.47\times10^{-11}$ F/m ($\varepsilon_0$ is the vacuum permittivity) are the permittivity of 1L and ML $MoS_2$, respectively [9]. $N_{\rm d1}$ and $N_{\rm dm}$ are the three-dimensional carrier densities. Using a simple model that the 2D carrier concentration is uniformly distributed along the vertical direction, from Section 1.1 and the thicknesses, we get $N_{\rm d1} = 10^{12}$ cm$^{-2}$/0.7 nm $= 1.4\times10^{25}$ m$^{-3}$ for the 1L and $N_{\rm dm} = 10^{12}$ cm$^{-2}$/$8\times0.7$ nm $= 1.8\times10^{24}$ m$^{-3}$ for the ML in Fig. 1c.

Provided the value of the built-in potential $qV_{\rm bi}$, the two unknown parameters, $x_1$ and $\phi_{\rm m}$, can be directly solved from equation (6) and (16). For $V_{\rm bi} = 0.10$ V (equation (3)), we obtain $x_1 = 1.2$ nm and $\phi_{\rm m} = 0.052$ V. The carrier density at the interface $N_{\rm di}$ is $n_{\rm m}(x=0) = N_{\rm dm}\exp(\frac{q\phi_{\rm m}}{k_{\rm B}T}) = 7.7\times N_{\rm dm} = 7.7\times10^{12}$ cm$^{-2}$. In analog to $p-n$ junctions, we use square waves to approximately describe the net charge density near the junction, shown in Fig. S5. We can estimate the width of the electron accumulation region on the ML side $x_{\rm m}$ using [8]

$$\phi_{\rm m} = q\frac{(N_{\rm di}-N_{\rm dm})x_{\rm m}^2}{2\varepsilon_{\rm m}} \tag{17}$$

The derived value is $x_{\rm m} = 2.3$ nm. The calculated parameters are summarized in Table S2.

Considering that the work functions of 1L and ML $MoS_2$ are not well-known parameters, we also calculate the interface parameters using $V_{\rm bi} = 0.15$ V and $V_{\rm bi} = 0.05$ V to estimate the influence of the $V_{\rm bi}$ value. The results are listed in Table S2. It was pointed out that, because of the weaker electron screening effect in a 2D material with respect to that in a 3D material, the interface electrons can spread over a wider range, i.e. a higher $x_{\rm m}$ and $x_1$ [10]. Our calculation may underestimate the $x_{\rm m}$ and $x_1$ values. Nevertheless, our $x_1$ value is in a reasonable agreement with the band profile directly imaged by STM at the $MoS_2$/graphene interface [11].

### S4.3 Conductance of the interface channel

Assuming a three-channel model of independent rectangular conducting channels, the conductance of the interface channel $G_{\mathrm{i}}$ can be extracted using

$$G = G_{\mathrm{m}} + G_1 + G_{\mathrm{i}} = \sigma_{\mathrm{m}}\frac{W_{\mathrm{m}}}{L} + \sigma_1\frac{W_1}{L} + G_{\mathrm{i}} \qquad (18)$$

where $W_{\mathrm{m}} = 5\ \mu$m, $W_1 = 4\ \mu$m, and $L = 7\mu$m are the width and length of the 1L and ML channels. The derived $G_{\mathrm{i}}$ ranges from 0.5 $\mu$S to 6 $\mu$S as a function of $V_{\mathrm{g}} = 0 - 40$ V. For comparison, the conductance of the ML channel is $G_{\mathrm{m}} = 0.02 - 3\ \mu$S for $V_{\mathrm{g}} = 0 - 40$ V. Considering that the ML channel is much wider than the interface region, the conductivity of the interface channel should be significantly higher than that of the ML.

### S4.4 Mobility of interface electrons

With the known interface carrier density $N_{\mathrm{di}}$ and the width of the electron accumulation region $x_{\mathrm{m}}$, the mobility of the interface electrons $\mu_{\mathrm{i}}$ can be calculated from the conductance of the interface channel using

$$G_{\mathrm{i}} = N_{\mathrm{di}} e \mu_{\mathrm{i}} \times \frac{x_{\mathrm{m}}}{L} \qquad (19)$$

where $L = 7\ \mu$m for the 1L/ML device in Fig. 1c.

Since $G$, $\sigma_1$ and $\sigma_{\mathrm{m}}$ are gate-voltage-dependent, the calculated $\mu_{\mathrm{i}}$ is also $V_{\mathrm{g}}$-dependent. For $V_{\mathrm{bi}} = 0.10$ V, $\mu_{\mathrm{i}} = 1300$ cm$^2$/Vs at $V_{\mathrm{g}} = 0$ V and $\mu_{\mathrm{i}} = 1.6 \times 10^4$ cm$^2$/Vs at $V_{\mathrm{g}} = 40$ V. For $V_{\mathrm{bi}} = 0.15$ V, $\mu_{\mathrm{i}}(V_{\mathrm{g}} = 0\ \mathrm{V}) = 970$ cm$^2$/Vs and $\mu_{\mathrm{i}}(V_{\mathrm{g}} = 40\ \mathrm{V}) = 1.1 \times 10^4$ cm$^2$/Vs. For $V_{\mathrm{bi}} = 0.05$ V, $\mu_{\mathrm{i}}(V_{\mathrm{g}} = 0\ \mathrm{V}) = 2900$ cm$^2$/Vs and $\mu_{\mathrm{i}}(V_{\mathrm{g}} = 40\ \mathrm{V}) = 2.5 \times 10^4$ cm$^2$/Vs. Besides the $V_{\mathrm{g}}$, the calculated $\mu_{\mathrm{i}}$ value also dependents on the value of carrier density $n$. Note that the $x_{\mathrm{m}}$ may be underestimated because of the weaker electron screening in the 2D case, the real values of $\mu_{\mathrm{i}}$ may be lower than the values presented here.

According to this simple heterostructure model, the interface electrons are accumulated at the 1L/ML interface with enhanced local carrier density and mobility. This model provides a possible explanation to the experimental results in Table S1 based on band bending. Other possible mechanisms, such as a possible edge state, are not considered here.


[1] Baugher, B. W. H., Churchill, H. O. H., Yang, Y. and Jarillo-Herrero, P. Intrinsic electronic transport properties of high-quality monolayer and bilayer $MoS_2$. *Nano Lett.* **13,** 4212-4216 (2013).

[2] Radisavljevic, B., Radenovic, A., Brivio, J., Giacometti, V. and Kis, A. Single-layer $MoS_2$ transistors. *Nature Nanotech.* **6,** 147-150 (2011).

[3] Kim, S., Konar, A., Hwang, W.-S., Lee, J., Yang, J., Jung, C., Kim, H., Yoo, J.-B., Choi, J.-Y., Jin, Y. W., Lee, S. Y., Jena, D., Choi, W and Kim, K. High-mobility and low-power thin-film transistors based on multilayer $MoS_2$ crystals. *Nature Comm.* **3,** 1011(2012).

[4] Radisavljevic, B. and Kis, A. Mobility engineering and a metalinsulator transition in monolayer $MoS_2$. *Nature Mater.* **12,** 815-820 (2013).

[5] Ghatak,S., Pal,A. N. and Ghosh, A. Nature of electronic states in atomically thin $MoS_2$ field-effect transistors. *ACS Nano*, **5,** 7707-7712(2011).

[6] Ochedowski, O., Marinov, K., Scheuschner, N., Poloczek, A., Bussmann, B. K., Maultzsch, J. and Schleberger, M. Effect of contaminations and surface preparation on the work function of single layer $MoS_2$. *Beilsterin J. Nanotechnol.* **5,** 291-297 (2014).

[7] Tosun, M.; Fu, D.; Desai, S. B.; Ko, C.; Kang, J. S.; Lien, D.-H.; Najmzadeh, M.; Tongay, S.; Wu, J.; Javey, A. $MoS_2$ heterojunctions by thickness modulation. *Sci. Rep.* DOI: 10.1038/srep10990 (2015).

[8] Sze, S. M. *Semiconductor Devices: Physics and Technology Ch. 4* (John Wiley and Sons, Inc, 2001).

[9] Cheiwchanchamnangij, T. and Lambrecht, W. R. L. Quasiparticle band structure calculation of monolayer, bilayer, and bulk $MoS_2$. *Phys. Rev. B* **85,** 205302(2012).

[10] Gurugubelli, V. K. and Karmalkar, S. Analytical theory of the space-charge region of lateral p-n junctions in nanofilms *J. Appl. Phys.* **118**, 034503 (2015).

[11] Zhang, C., Johnson, A., Hsu, C-L., Li, L-J and Shih, C-K. Direct imaging of band profile in single layer $MoS_2$ on graphite: quasiparticle energy gap, metallic edge states, and edge band bending *Nano Lett.* **14,** 2443-2447 (2014).
